# Supplementary material for: Probing the Quantum and Classical Boundary: A Tabletop Experiment Using Quantum Optics
Source: arXiv:2411.10347 source file (2024-11-15)
Supplement: Supplementary file 1 [file Appendix_DoubleslitCalc.tex]

\section{Response Time of a SPDC}

Let us consider a $1+1$-Dimensional theory, and demonstrate that an SPDC does not theoretically have a response time needed. For the SPCD process in $1+1$ dimensions, we may write the wave-equation \cite{SPDCTheoryReview}:
\begin{align}
    \frac{\partial^2 E}{\partial^2 x} - \frac{\partial^2 E}{\partial^2 t} = \frac{1}{\epsilon_0^2} \frac{\partial^2}{\partial t} E^2
\end{align}
For easiness of notation, all of our calculation in this section will be in natural units. The right hand side corresponds to an interaction term, and the left hand side is generated by the free Lagrangian:
\begin{align}
    \mathcal{L}_{f} = \frac{1}{2} \partial^{\mu}\partial_{\mu} E
\end{align}
Let us now work backwords. We guess that the $SPDC$ is fundamentally a $3$ photon process, thus we take:
\begin{align}
    L_{int} = \frac{1}{3!}g^3 E^3
\end{align}

\section{Muchen's Calculation Attempt}
Consider the single slit case. Let us assume $f_0$ is much greater than the slit size. Then, the diffraction patter from either slit can be though of as a single slit diffaction on the screen.

\section{Hery's Calculation Attempt}
To calculate the coherent image obtained during the actual measurements of the experiment, we consider the following:

The wave function after BBO is

\begin{align}
    \ket{\psi} \frac{1}{\sqrt{2}} \
\end{align}

When forming a classical measurement, the function of the sample number is

\begin{align}
    R(t_{0},t_{1}) \propto \bra{0}E_{1}^{(+)}E_{0}^{(+)} \ket{\psi}
\end{align}

According to Scully's calculation \cite{PhysRevLett.75.4337}, we have

\begin{align}
    R \propto \Pi(t_{0}-t_{1})e^{-i \omega_{s}t_{0}}e^{-i \omega_{i} t_{1}}
\end{align}

which is shown that there is only one amplitude and no interference is expacted.

To calculate the intensity distribution of the double-slit interference pattern, we typically follow these steps based on the principles of wave interference:

Suppose light waves emitted from two slits (A and B) meet at a point \(P\). The wave equations can be expressed as:

\begin{align}
    E_A = E_0 e^{i(kx_A - \omega t)} \\
    E_B = E_0 e^{i(kx_B - \omega t)}
\end{align}

where \(E_0\) is the amplitude of the light wave, \(k = \frac{2\pi}{\lambda}\) is the wave number, and \(\omega\) is the angular frequency.

The phase difference \(\Delta \phi\) at point \(P\) is determined by the path difference \(\Delta d\) between the waves:

\begin{align}
    \Delta \phi = k \Delta d = \frac{2\pi}{\lambda} \Delta d
\end{align}

The total electric field from both waves can be expressed as:

\begin{align}
    E_{total} = E_A + E_B = E_0 e^{i(kx_A - \omega t)} + E_0 e^{i(kx_B - \omega t)}
\end{align}

Factoring out the common term:
\begin{align}
    E_{total} = E_0 e^{-i\omega t} \left( e^{ikx_A} + e^{ikx_B} \right)
\end{align}

The intensity \(I\) is proportional to the square of the total electric field:
\begin{align}
    I \propto |E_{total}|^2 = |E_0|^2 |e^{ikx_A} + e^{ikx_B}|^2
\end{align}

Calculating the modulus squared:
\begin{align}
    &|e^{ikx_A} + e^{ikx_B}|^2 = |e^{ikx_A}|^2 + |e^{ikx_B}|^2 \notag \\
    &+ 2 \text{Re}\{e^{ikx_A} e^{-ikx_B}\} = 1 + 1 + 2\cos(\Delta \phi)
\end{align}

Therefore:
\begin{align}
    I \propto 2 |E_0|^2 (1 + \cos(\Delta \phi))
\end{align}

Substitute the expression for the phase difference \(\Delta \phi\) in terms of the path difference:

\begin{align}
I \propto 2 |E_0|^2 \left(1 + \cos\left(\frac{2\pi}{\lambda} \Delta d\right)\right)
\end{align}
